# Supplementary material for: GenCorres: Consistent Shape Matching via Coupled Implicit-Explicit Shape Generative Models
Source: arXiv:2304.10523 source file (2024-04-16)
Supplement: Supplementary file 1 [file 9_appendix.tex]

\newpage
\newpage
\newpage
\section{Expression of $\overline{L}^{\arap}(g^{\phi}(\bs{z}))$}
\label{Sec:L:ARAP:Expression}

where
$$
\overline{L}^{\arap}(\bs{g}^{\phi}(\bs{z})) = L\otimes I_3 - B^{\arap}\big(\bs{g}^{\phi}(\bs{z})\big)D^{\arap}\big(\bs{g}^{\phi}(\bs{z})\big){B^{\arap}\big(\bs{g}^{\phi}(\bs{z})\big)}^T
$$
where $L$ is the graph Laplacian of the mesh, and $B^{\arap}\big(\bs{g}^{\phi}(\bs{z})\big)\in \R^{3n\times 3n}$ is a sparse block matrix defined as
$$
B^{\arap}_{ij}\big(\bs{g}^{\phi}(\bs{z})\big)  = \left\{
\begin{array}{cc}
\sum\limits_{j'\in \set{N}_i}\bs{e}_{ij}^{\phi}(\bs{z}) \times  & i = j \\
-\bs{e}_{ij}^{\phi}(\bs{z}) \times  & j\in \set{N}_i \\
 0 & \textup{else}
\end{array}
\right. 
$$
where $\bs{e}_{ij}^{\phi}(\bs{z}) =\bs{g}_i^{\phi}(\bs{z})-\bs{g}_j^{\phi}(\bs{z})$ and $D^{\arap}\big(\bs{g}^{\phi}(\bs{z})\big)\in \R^{3n\times 3n}$ is a diagonal block matrix defined as 
$$
D^{\arap}_{ii}\big(\bs{g}^{\phi}(\bs{z})\big)  =
\Big(\sum\limits_{j\in \set{N}_i}\big(\|\bs{e}_{ij}^{\phi}(\bs{z}) \|^2 I_3-\bs{e}_{ij}^{\phi}(\bs{z}) {\bs{e}_{ij}^{\phi}(\bs{z})} ^T\big)\Big)^{-1}
$$

\section{Expression of $\overline{L}^{\acap}(g^{\phi}(\bs{z}))$}
\label{Sec:L:ACAP:Expression}

$$
\overline{L}^{\acap}(\bs{g}^{\phi}(\bs{z})) = L\otimes I_3 - B^{\acap}\big(\bs{g}^{\phi}(\bs{z})\big)D^{\acap}\big(\bs{g}^{\phi}(\bs{z})\big){B^{\acap}\big(\bs{g}^{\phi}(\bs{z})\big)}^T
$$
where $B^{\acap}\big(\bs{g}^{\phi}(\bs{z})\big)\in \R^{3n\times 4n}$ is a sparse block matrix defined as
$$
B^{\acap}_{ij}\big(\bs{g}^{\phi}(\bs{z})\big)  = \left\{
\begin{array}{cc}
\sum\limits_{j'\in \set{N}_i}\big(\begin{array}{cc}
-\bs{e}_{ij}^{\phi}(\bs{z}) & \bs{e}_{ij}^{\phi}(\bs{z}) \times
\end{array}\big)  & i = j \\
\big(\begin{array}{cc}
\bs{e}_{ij}^{\phi}(\bs{z}) & -\bs{e}_{ij}^{\phi}(\bs{z}) \times
\end{array}\big)
&j\in \set{N}_i \\
 0 & \textup{else}
\end{array}
\right. 
$$
and $D^{\acap}\big(\bs{g}^{\phi}(\bs{z})\big)\in \R^{4n\times 4n}$ is a diagonal block matrix defined as 
$$
D^{\acap}_{ii}\big(\bs{g}^{\phi}(\bs{z})\big)  =
\Big(\sum\limits_{j\in \set{N}_i}\big(\|\bs{e}_{ij}^{\phi}(\bs{z}) \|^2 I_4-\diag(0,\bs{e}_{ij}^{\phi}(\bs{z}) {\bs{e}_{ij}^{\phi}(\bs{z})} ^T\big)
\Big)^{-1}
$$

\section{Training Procedure for Learning the Implicit Generator}
\label{Section:Training:Implicit:Generator}

\noindent\para{Pose initialization.}
%\label{Subsecsec:Variable:Initialization}
We initialize the rigid object poses $T_i$ by adopting a state-of-the-art pose synchronization technique~\cite{Huang_2019_CVPR}. This is done by first establishing a graph among the input objects by connecting each shape with $k$-nearest neighbors ($k=20$ in all of our experiments) with respect to the D2 shape descriptor~\cite{10.1145/571647.571648}, which can identify approximately similar shapes. For each edge $(S_i,S_j)$ of this shape graph, we apply \qixing{TBD} to predict a relative rigid pose $T_{ij}\in SE(3)$ between $S_i$ and $S_j$. We use \qixing{TBD} over other methods, as it is stable against approximate and partial rigid invariance. We then fit the relative rigid poses $T_{ij}$ into ~\cite{Huang_2019_CVPR}, which outputs consistent absolute poses $T_i$ of the input shapes. Our experiments show that the maximum error among the estimated absolute poses $T_i$ is below $30^{\circ}$ for all the datasets we have tested, which is sufficient for pose initialization (See Figure~\ref{Figure:Absolute:Pose:Error}). 
\begin{figure}[h]
\centering
\vspace{1.25in}
\caption{Plots on the absolute rotational errors of the three category of datasets tested in this paper. (Left) Human. (Middle) Animal. (Right) Bone.}
\label{Figure:Absolute:Pose:Error}
\end{figure}

Following~\cite{Huang_2021_ICCV}, we initialize the latent variables $\{\bs{z}_i,1\leq i \leq N\}$ by performing principal component analysis (PCA) of the D2 shape descriptors. The latent code $\bs{z}_i$ of $S_i$ is initialized as the $i$-th elements of the first $d$ eigenvectors of the PCA matrix. 

Following~\cite{Huang_2021_ICCV}, we drop the regularization terms in (\ref{Eq:Implicit:Loss:Term}) to minimize the data term to initialize the network parameters $\phi$:
$$
\phi^{\init} = \underset{\phi}{\textup{argmin}} \sum\limits_{i=1}^{N}\frac{1}{n_i}\sum\limits_{j=1}^{n_i}\big(g^{\phi}(T_i(\bs{s}_{ij}), \bs{z}_i)-d_{ij}\big)^2.
$$
This amounts to solving the standard network training problem of implicit generators, which employs ADAM~\cite{DBLP:journals/corr/KingmaB14} for optimization. 

\noindent\para{Training procedure.} We apply

Starting from the initial variables, we proceed to solve (\ref{Eq:Implicit:Loss:Term}) via alternating minimization. When $\bs{z}_i$ and $T_i$ are fixed, (\ref{Eq:Implicit:Loss:Term}) reduces to 
$$
\min\limits_{\phi}\frac{1}{N}\frac{1}{n_i}\sum\limits_{j=1}^{n_i} \big(g^{\phi}(T_i(\bs{s}_{ij}), \bs{z}_i)-d_{ij}\big)^2 + \lambda_{\geo}r_{\geo}(g^{\phi}) + \lambda_{\cycle}r_{\cycle}(g^{\phi})
$$
which is solved via ADAM~\cite{DBLP:journals/corr/KingmaB14}. Gradient computation applies and its extension to the cycle-consistency regularization term, which result in derivatives of the loss with respect to each $\bs{g}^{\phi}_i(\bs{z})$. The derivative of $\bs{g}^{\phi}_i(\bs{z})$ with respect to $\phi$ is given by
\begin{equation}
\frac{\partial \bs{g}_i^{\phi}(\bs{z})}{\partial \phi} = -{\frac{\partial g^{\phi}}{\partial \bs{x}}(\bs{g}_i^{\phi}(\bs{z}),\bs{z})}^T\frac{\partial g^{\phi}}{\partial \phi}(\bs{g}_i^{\phi}(\bs{z}),\bs{z})). 
\label{Eq:Chain:Rule}
\end{equation}

When $\bs{z}_i$ and $\phi$ are fixed, (\ref{Eq:Implicit:Loss:Term}) reduces to performing rigid registration under implicit surface representations:
\begin{equation}
\min\limits_{T_i} \sum\limits_{j=1}^{n_i} \big(g^{\phi}(T_i(\bs{s}_{ij}), \bs{z}_i)-d_{ij}\big)^2.
\label{Eq:Implicit:Rigid:Registration}
\end{equation}
We solve (\ref{Eq:Implicit:Rigid:Registration}) via Gauss-Newton method. Denote the current location $\bs{s}_{ij}$ as $\bs{s}_{ij}^{\textup{c}} = T_i(\bs{s}_{ij})$. We optimize the velocity vectors $\bs{c}_i$ and $\overline{\bs{c}}_i$ for the rotation and translation components of $T_i$ via
$$
\min\limits_{\bs{c}_i,\overline{\bs{c}}_i} \sum\limits_{j=1}^{n_i} \big(g^{\phi}(\bs{s}_{ij}^{\textup{c}}, \bs{z}_i)-d_{ij} + {\frac{\partial g^{\phi}}{\partial \bs{x}}}^T(\bs{s}_{ij}^{\textup{c}})(\bs{c}_i\times\bs{s}_{ij}^{\textup{c}} + \overline{\bs{c}}_i)\big)^2.
$$
We then update the rotation component $R_i$ and the translation component $\bs{t}_i$ of $T_i$ via $R_i\leftarrow \exp(\alpha_i\bs{c}_i\times)R_i$ and $\bs{t}_i\leftarrow \bs{t}_i + \alpha_i\overline{\bs{c}}_i$ where step-size $\alpha_i$ is determined via line search. 

Finally, when $T_i$ and $\theta$ are fixed, (\ref{Eq:Implicit:Loss:Term}) reduces to
\begin{equation}
\min\limits_{\{\bs{z}_i\}} \frac{1}{N}\sum\limits_{i=1}^{N}\frac{1}{n_i}\sum\limits_{j=1}^{n_i} \big(g^{\phi}(T_i(\bs{s}_{ij}), \bs{z}_i)-d_{ij}\big)^2 + \lambda_{\KL}\KL(\set{N}_d,\{\bs{z}_i\}).
\label{Eq:Latent:Code:Opt}    
\end{equation}
We solve (\ref{Eq:Latent:Code:Opt}) via ADAM~\cite{DBLP:journals/corr/KingmaB14}. Our implementation applies four iterations of alternating minimizations. 

\section{Template Based Registration}
\label{Sec:Template:Based:Registration}

\section{Mesh Generator Architecture}
\label{Sec:Explicit:Network:Architecture}

The network architecture of $\bs{g}^{\theta}$ follows from that in~\cite{Huang_2021_ICCV}, which outputs displacements of vertex positions of the template mesh $S_1$. We sample 4 resolutions of the mesh connections of the template mesh.  The network architecture stacks 4 blocks of convolution + up-sampling layers. The convolution layer employs Chebyshev convolutional filters with $K = 6$ Chebyshev polynomials~\cite{ranjan2018generating}. Similar to~\cite{zhou2020fully}, there is a fully connected layer between the latent code and the input to the first convolution layer. 

\section{Training Details of the Mesh Generator}
\label{Section:Mesh:Training:Details}

Given a template mesh $S_1$, we seek to find corresponding vertices of $S_1$ on other training shapes. This is done by constructing a spanning tree $\set{T}$ rooted at $S_1$ among the input shapes that connects shapes with adjacent shapes and recursively computing correspondences along edges of $\set{T}$ to propagate correspondences of $S_1$ to other shapes. Specifically, along each edge $(S_i,S_j)$ of $\set{T}$ where we have correspondences of $S_1$ on $S_i$, we sample $l$ ($l=10$ in our experiments) intermediate shapes $\bs{z}_{ij,k}= \bs{z}_i + \frac{k}{l+1}(\bs{z}_j-\bs{z}_i),0\leq k \leq l+1$. We then apply (\ref{Eq:Displacement:Defn}) to progressively propagate correspondences from implicit surface $g^{\phi}(\bs{x},\bs{z}_{ij,k}) = 0$ to the next implicit surface $g^{\phi}(\bs{x},\bs{z}_{ij,k+1}) = 0$. As the implicit generator is trained to prioritize that the induced correspondences are cycle-consistent, we find that the propagated correspondences are insensitive to different choices of the spanning tree. 

Given the propagated dense correspondences $\bs{g}_1^{\init}$ from the template mesh $S_1$ and other shapes $S_i$, we initialize $\bs{g}^{\theta}$ via standard regression, i.e.,
$$
\theta^{\init} = \underset{\theta}{\textup{argmin}}\sum\limits_{i=1}^{N} \|\bs{g}_i^{\init}-\bs{g}^{\theta}(\bs{z}_i)\|^2.
$$

\section{Details of the Dataset}
\label{Section:Appendix:Dataset}
