# Supplementary material for: GenCorres: Consistent Shape Matching via Coupled Implicit-Explicit Shape Generative Models
Source: arXiv:2304.10523 source file (2024-04-16)
Supplement: Supplementary file 2 [file _main_supp.tex]

\documentclass[10pt,twocolumn,letterpaper]{article}

\usepackage{iccv}
\usepackage{times}
\usepackage{epsfig}
\usepackage{graphicx}
\usepackage{amsmath}
\usepackage{amssymb}
\usepackage{multirow}
\usepackage{multicol}
\usepackage{booktabs}
\usepackage{overpic}
% Include other packages here, before hyperref.

% If you comment hyperref and then uncomment it, you should delete
% egpaper.aux before re-running latex.  (Or just hit 'q' on the first latex
% run, let it finish, and you should be clear).
\usepackage[pagebackref=true,breaklinks=true,letterpaper=true,colorlinks,bookmarks=false]{hyperref}

% \iccvfinalcopy % *** Uncomment this line for the final submission

 % *** Enter the ICCV Paper ID here

\usepackage{wrapfig}

\input{macros.tex}
% Pages are numbered in submission mode, and unnumbered in camera-ready
\ificcvfinal\pagestyle{empty}\fi

\begin{document}

%%%%%%%%% TITLE
\title{GenCorres: Consistent Shape Matching via Coupled Implicit-Explicit Shape Generative Models -- Supplementary Material}

\maketitle
% Remove page # from the first page of camera-ready.
\ificcvfinal\thispagestyle{empty}\fi

%\begin{teaserfigure}
%\vspace{1.65in}
%\caption{(Left) GenCorres learns an implicit generator from a collection of unorganized shape collections. We introduce a novel approach to compute correspondences between two neighboring implicit surfaces. The resulting correspondences are forced to be as-rigid-as possible or as-conformal-as possible and cycle-consistent among triplets of neigboring shapes. These two constraints are enforced as regularization terms to train the generator. (Right) The resulting generator offers high-quality inter-shape correspondences by composing correspondences along a path of of intermediate shapes.}
%\Description{figure description}
%\label{Figure:Teaser}
%\end{teaserfigure}

%%%%%%%%% ABSTRACT

%%%%%%%%% BODY TEXT
\input{supp/0_intro}
\input{supp/1_reg_loss}
\input{supp/2_mesh_gen_init}
\input{supp/3_dataset}
\input{supp/4_shape_space}
\input{supp/5_correspondence}

{\small
\bibliographystyle{ieee_fullname}
\bibliography{ref,matching,haitao}
}

\newpage
\appendix
\end{document}
